# Supplementary material for: Nanomechanical detection of the spin Hall effect
Source: arXiv:1509.01269 source file (2016-05-09)
Supplement: Supplementary file 1 [file Supplement.pdf]

# Supplementary Material to: Nanomechanical detection of the spin Hall effect

J. A. Boales, C. T. Boone, and P. Mohanty
*Department of Physics, Boston University, 590 Commonwealth Avenue, Boston, MA 02215*

## FORCE DISTRIBUTION

Since COMSOL Multiphysics does not allow a torque density to be applied to a material, we derive an approximately equivalent form of the torque density using force couples. The net torque on one half of the oscillator must be the same using both formulations. The net force on each half of the oscillator must also be zero. The forces are applied along the length of the wire. To begin, we write down a formula for the net torque about the z-axis on the left side of the wire

$$T_z = \int\limits_{\text{left half}} \tau_z \, dV = Lh \int\limits_{-w/2}^{0} \tau_z \, dx \qquad \text{(SM-1a)}$$

where $\tau_z$ is the torque density about the $z$-direction, $L$ is the length, $h$ is the thickness, and $w$ is the width of the wire. Equivalently, we write this as an integral over a continuum of force couples

$$T_z = Lh \int_{-w/2}^{0} \left(\frac{w}{2} - |x|\right) f_{y,z} \, dx \qquad \text{(SM-1b)}$$

where $f_{y,z}$ refers to some unknown force density distribution in the $y$-direction due to the torque density distribution $\tau_z$. This leads to the conclusion that

$$f_{y,z} = \frac{|\tau_z|}{w/2 - |x|}. \qquad \text{(SM-1c)}$$

This method is similarly used to derive a force density distribution $f_{y,x}$ oriented in the $y$-direction to emulate the torque density distribution $\tau_x$ about the $x$-direction

$$f_{y,x} = \frac{|\tau_x|}{h/2 - |z|}. \qquad \text{(SM-1d)}$$

These force density distributions are balanced by forces applied to the boundaries of the wire

$$F_{y,\text{left/right}} = -\int\limits_{\text{left half}} f_{y,x} \, dV \qquad \text{(SM-1e)}$$

$$F_{y,\text{top/bottom}} = -\int\limits_{\text{top half}} f_{y,z} \, dV \qquad \text{(SM-1f)}$$

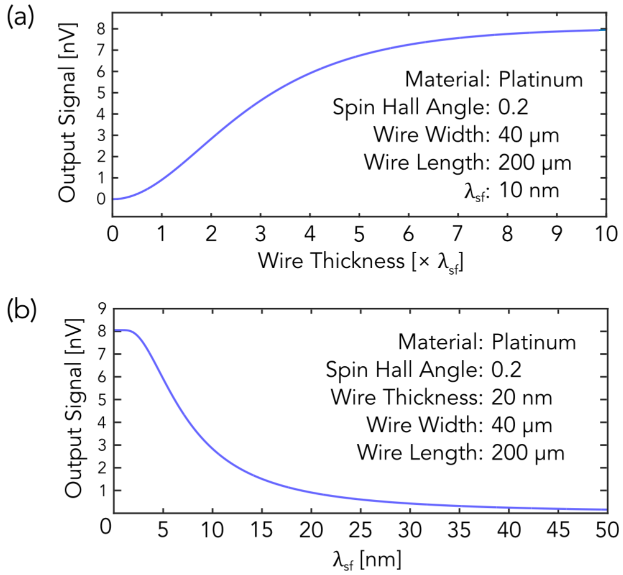


FIG. SM-1. **(a)** Variation of DC output signal with wire thickness (in units of $\lambda_{sf}$). **(b)** Variation of DC output signal with $\lambda_{sf}$.

## DC SIGNAL DEPENDENCE

Figure SM-1a illustrates the DC output signal variation with wire thickness, and Figure SM-1b illustrates the DC output signal variation with spin flip length. In both subfigures, a 1 mV potential is applied to the wire. Using the COMSOL model, we found that there is an approximately linear relationship between the torque due to the spin accumulation on the top and bottom surfaces of the wire and the output signal as follows:

$$T_x = \left(3.08 \times 10^{-18}\ \text{N} \cdot \text{m/nV}\right) \cdot V_{\text{out}} \qquad \text{(SM-2)}$$

Using the characteristic curves in Figures SM-1a and SM-1b along with the calibration curve in Eq. SM-2, it is possible to determine the spin diffusion length and spin Hall angle experimentally. As shown in Figure SM-1a, when the wire thickness is greater than about $8\lambda_{sf}$, the output signal plateaus. By performing the experiment using different wire thicknesses and fitting to this characteristic curve, we can determine the spin diffusion length. With this experimental setup, the thickness of the wire is easily controlled and measured, making it an ideal parameter to be used in determining these fundamental spin properties.

## SENSITIVITY ANALYSIS

Here we present the details of the noise analysis used to determine the predicted sensitivity of our experimental setup.

### *Thermal Johnson Noise*

To evaluate the thermal Johnson noise, we construct a simple damped harmonic oscillator equivalent system

$$M\ddot{x} + M\gamma\dot{x} + Kx = F(t) \qquad \text{(SM-3)}$$

where $M$ is the equivalent mass of the system, $\gamma$ is the damping factor, $K$ is the equivalent stiffness, $x(t)$ is a translational degree of freedom, and $F(t)$ is a time-varying applied force. $\gamma$ can be equivalently written as $\omega_0/Q$, where $\omega_0$ is the resonant frequency and $Q$ is the quality factor (100, in this case). Taking the Fourier transform, this can be rewritten as

$$|X(\omega)| = \frac{|F(\omega)|}{M\sqrt{(\omega^2 - \omega_0^2)^2 + \gamma^2\omega^2}}. \qquad \text{(SM-4)}$$

For an oscillator driven at peak frequency by a sinusoidal force, the peak response becomes

$$|X(\omega_0)| = \frac{F_0}{M\gamma\omega_0}. \qquad \text{(SM-5)}$$

Since, in its 19.18 MHz mode, the bulk of the beam translates along the length of the beam, we assert that the mass of the equivalent mass of the beam is approximately the actual mass of the beam, or $2 \times 10^{-10}$ kg. Using this, and knowing that $f_0$ is 19.18 MHz and $Q$ is 100, we find that the appropriate values for $K$ and $\gamma$ are $2.905 \times 10^6$ N/m and $1.205 \times 10^6$ s$^{-1}$, respectively.

Using this calculated value of $K$ and the fact that, for DC currents, the maximum displacement of the beam is about 0.28 fm/mA, we find that the magnitude of the equivalent force we apply is $F_0 = 2.904 \times 10^{-11}$ N, producing a maximum displacement of 1.0 fm.

Replacing the sinusoidal force with the thermal Johnson force $\sqrt{4k_BTM\gamma}$, again applied at resonance, the displacement due to Johnson noise is

$$\sqrt{\langle x^2 \rangle} = \frac{\sqrt{4k_BTM\gamma}}{M\gamma\omega_0}. \qquad \text{(SM-6)}$$

At 300 K, this corresponds to about 0.069 fm/$\sqrt{\text{Hz}}$ of random motion, or 92.3 nV of noise on the signal for a 20 Hz bandwidth. At 4 K, the random motion is reduced to 0.0079 fm/$\sqrt{\text{Hz}}$, or 10.7 nV of noise on the signal.

### *Capacitive Johnson Noise*

At resonance, the spectral density of the capacitive Johnson noise is

$$S^{\text{cap}} = 4k_BT \ \text{Re}[Z]. \qquad \text{(SM-7)}$$

Here, we model the electrical portion as an RC circuit. As such, the real part of the impedance is simply the 50-Ω impedance of the connections. For a 20 Hz measurement bandwidth, we can expect 0.47 nV of noise.

### *Preamplifier noise*

The presence of a preamplifier will produce a small amount of noise on the signal. For this calculation we assert that the preamplifier produces 1 nV/$\sqrt{\text{Hz}}$ of noise. For a 20 Hz measurement bandwidth, we can expect 4.47 nV of noise.

### *Shot Noise*

We anticipate a small amount of shot noise due to the flow of current through the wire that crosses the beam. The spectral density for shot noise is

$$S^{\text{shot}} = 2e|I|. \qquad \text{(SM-8)}$$

In the experiment described in this paper, the current is about 35 $\mu$A, giving a spectral density $1.12 \times 10^{-15}$ V$^2$/Hz. Using a measurement bandwidth of 20 Hz, we can anticipate 15 pV of input noise, or $4.49 \times 10^{-6}$ nV of shot noise on the output.

### *Summary*

At room temperature, the primary contribution to the experimental noise comes from thermal Brownian motion, followed by noise due to the preamplifier. Including all types presented here, the anticipated noise at room temperature is approximately 92.5 nV. At 4 K, thermal noise still dominates, though at a much lower level. The anticipated noise from all sources is 11.6 nV.

TABLE SM-I. Summary of MEMS parameters used in the simulations.

| **Parameter** | **Variable** | **Value** |
|---|---|---|
| Young's Modulus - Pt | $E_{\mathrm{Pt}}$ | 168 GPa |
| Poisson's ratio - Pt | $\varepsilon_{\mathrm{Pt}}$ | 0.38 |
| Electrical Conductivity - Pt | $\sigma$ | $8.9 \times 10^6$ S/m |
| Young's Modulus - Si | $E_{\mathrm{Si}}$ | 160 GPa |
| Poisson's Ratio - Si | $\varepsilon_{\mathrm{Si}}$ | 160 GPa |
| Si Thickness | $t_{\mathrm{Si}}$ | 5 $\mu$m |
| Young's Modulus - $SiO_2$ | $E_{\mathrm{SiO^2}}$ | 70 GPa |
| Poisson's Ratio - $SiO_2$ | $\varepsilon_{\mathrm{SiO_2}}$ | 0.17 |
| $SiO_2$ Thickness | $t_{\mathrm{SiO_2}}$ | 1 $\mu$m |
| Young's Modulus - Mo | $E_{\mathrm{Mo}}$ | 312 GPa |
| Poisson's Ratio - Mo | $\varepsilon_{\mathrm{Mo}}$ | 0.30 |
| Mo Thickness | $t_{\mathrm{Mo}}$ | 600, 600 nm |
| AlN Thickness | $t_{\mathrm{AlN}}$ | 2 $\mu$m |
| Beam Width | $w$ | 40 $\mu$m |
| Beam Length | $L$ | 200 $\mu$m |
